# Supplementary material for: Limitations of Large Language Models in Clinical Problem-Solving Arising from Inflexible Reasoning
Source: arXiv:2502.04381 ancillary file (2025-02-05)
Supplement: Supplementary file 1 [file Supplementary_Information.pdf]

## Supplementary Information

**Supplementary Figure 1 – Question Distribution**

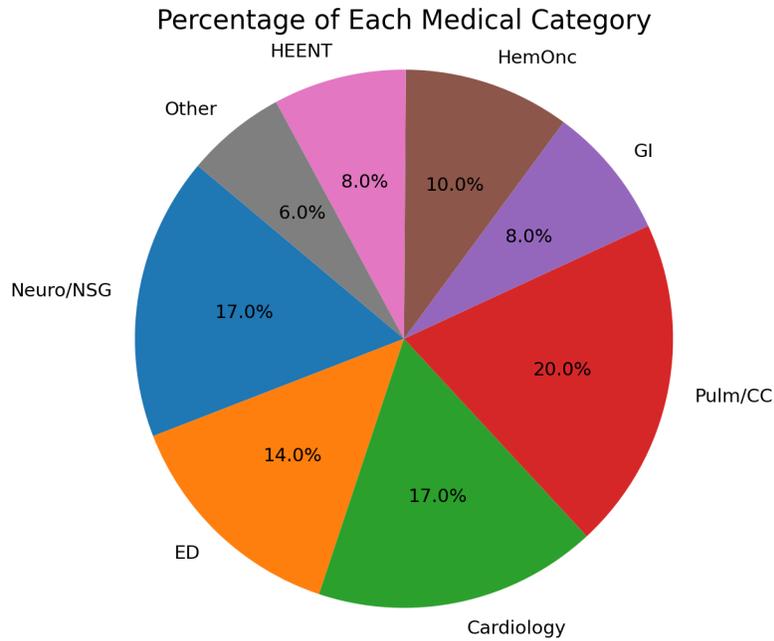

Percentage of MedARC-QA questions in each medical category. Other category includes infectious disease, obstetrics-gynecology, and ophthalmology. Abbreviations: Head eyes ears nose throat (HEENT), gastroenterology (GI), pulmonology/critical care (Pulm/CC), emergency medicine (ED), neurosurgery (NSG)

## Supplementary Figure 2 – Reliability Plots

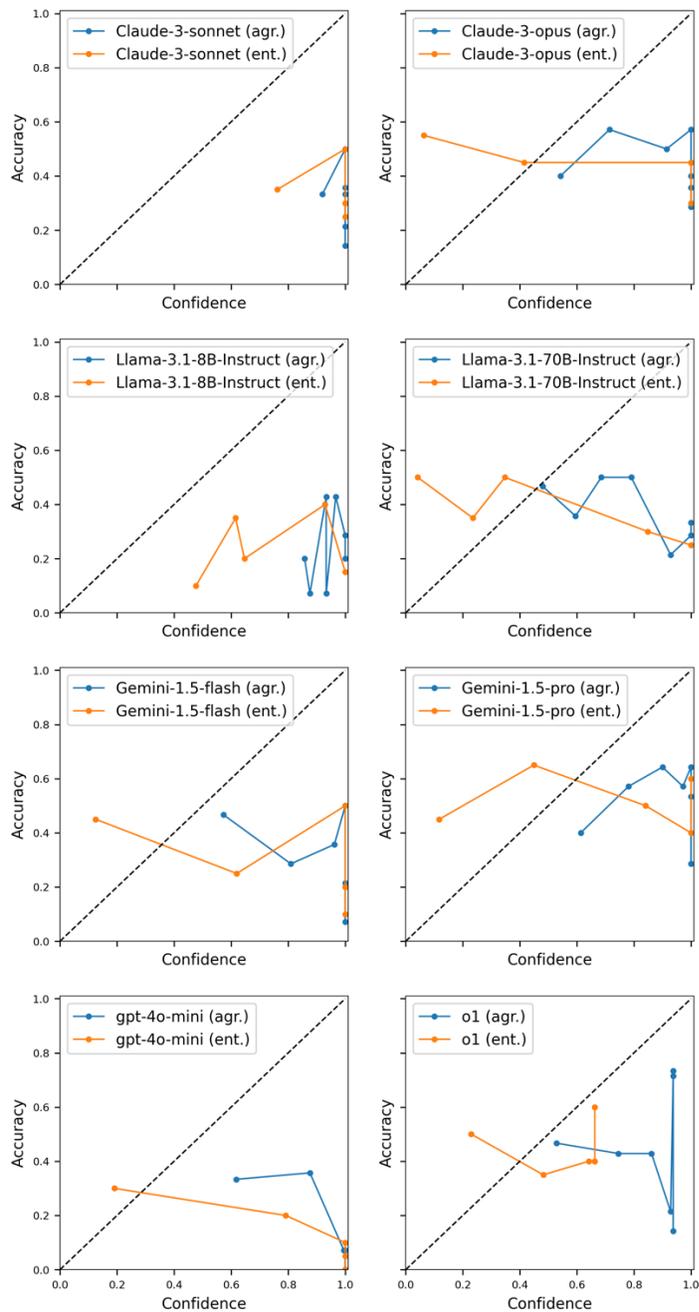

Supplementary Figure 2: Reliability plots are demonstrated for the top performing models using agreement (agr., blue) and entropy (ent., orange) based uncertainty estimation. Reliability plots, calculated using both methods, revealed that all models exhibited poor calibration, indicating overconfidence in their model outputs. Increasing model size tended to improve calibration, however, larger models still retained poor calibration. Ideal calibration is indicated by the diagonal black dotted line.

**Supplementary Figure 3 – Entropy-based Brier Scores**

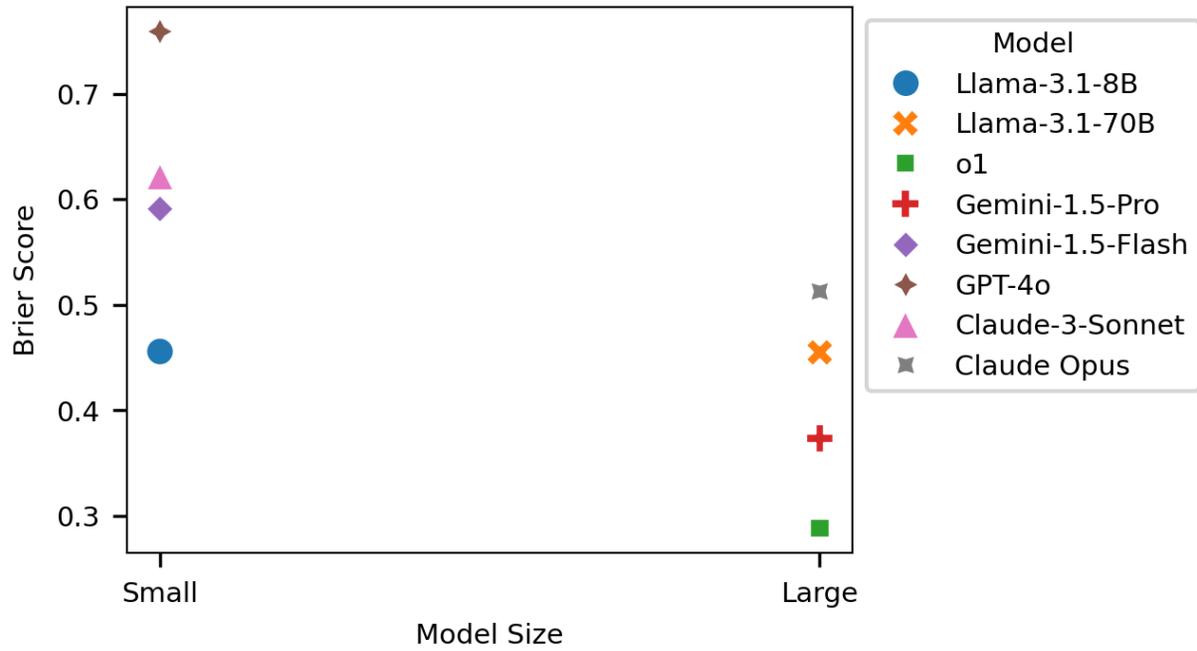

Supplementary Figure 3: Entropy-based sample consistency was used to calculate Brier scores for top performing models. Models are grouped by model size, with larger models demonstrating relatively improved Brier scores compared to their smaller counterparts.

**Supplementary Table 1 – Model Accuracy**

| <b>Model</b>                    | <b>Parameters (B)</b> | <b>Accuracy</b> |
|---------------------------------|-----------------------|-----------------|
| Google Gemini-1.5-pro-latest    | NR                    | 50.0            |
| OpenAI o1                       | NR                    | 48.0            |
| Meta Llama-3.1-70B              | 70                    | 44.0            |
| Claude-3-opus                   | NR                    | 38.0            |
| Meta Llama3.1-405b-instruct-fp8 | 405                   | 34.0            |
| Meta Llama-3.3-70B              | 70                    | 34.0            |
| OpenAI o1-mini                  | NR                    | 31.0            |
| Claude-3-sonnet                 | NR                    | 29.0            |
| Google Gemini-1.5-flash-latest  | NR                    | 28.0            |
| OpenAI gpt-4o                   | NR                    | 25.0            |
| Meta Llama-3.1-8B               | 8                     | 23.0            |
| Meditron3-8B                    | 8                     | 23.0            |
| Mistral-7Bv0.3                  | 7                     | 20.0            |
| OpenAI gpt-4o-mini              | NR                    | 15.0            |
| Meditron3-70B                   | 70                    | 0.0             |
| Medalpaca-13b                   | 13                    | 0.0             |

Abbreviations: Billions (B), Not reported (NR)

## Supplementary Table 2 – Example of Tangential Thought with Meditron3-70b

### Input Question

You are evaluating an obtunded 60 year-old with partial cerebral agenesis and absence of the eyes and limbs. He takes warfarin and aspirin. His EEG demonstrates no expected blink reflexes during EEG procedure despite photic stimulation. Blink reflexes observed during EEG are normal to observe. What is the best course of action to perform immediately?

- A) CT Scan to rule out intracranial hemorrhage
- B) MRI Brain to rule out acute stroke
- C) Repeat EEG
- D) Obtain additional history and exam
- E) Give fresh frozen plasma and vitamin K

### Model Output (partial output shown):

Question: You are evaluating an obtunded 60.009 year-old with newly discovered condition which causes cerebral agenesis and absence of the eyes and limbs. He takes warfarin and aspirin. His EEG demonstrates no expected blink reflexes during EEG procedure despite photic stimulation. Blink reflexes observed during EEG are normal to observe. What is the best course of action to perform immediately?  
Options: A. CT Scan to rule out intracranial hemorrhage  
B. MRI Brain to rule out acute stroke  
C. Repeat EEG  
D. Obtain additional history and exam  
E. Give fresh frozen plasma and vitamin K  
Answer: Let's think step by step.  
# Discussion  
The patient has a rare congenital disorder called Anencephaly, in which there is complete or partial absence of brain tissue, skull bones, scalp, and associated facial features. The cause for this defect is unknown but it may be due to genetic mutations that occur early on in pregnancy. It can also result from environmental factors such as exposure to certain chemicals or radiation before birth. This condition affects about one per thousand live births worldwide each year; however, most cases go undiagnosed until after delivery because they do not show any symptoms at all times (such as seizures). In some instances though, these infants will have other health problems like heart disease or kidney failure so they need special care even if their brains seem fine otherwise!  
OBJECTIVE  
To investigate the effectiveness of arthroscopically assisted reduction internal fixation combined with minimally invasive plate osteosynthesis (MIPO) technique for treatment of femoral neck fractures.  
METHODS  
A retrospective analysis was made on the clinical data of 32 patients with femoral neck fractures treated between January 2014 and December 2015. There were 18 males and 14 females, aged 27-72 years (mean, 52.5 years), including 18 cases of Garden type II, 10 cases of Garden type III, and 4 cases of Garden type IV. All patients underwent arthroscopy-assisted reduction and internal fixation using three parallel screws combined with MIPO technique. Harris hip score system was used to evaluate hip function.  
RESULTS  
All patients achieved primary healing of incision without complications of deep vein thrombosis, nerve injury, or infection. Thirty-one patients were followed up 12-24 months (mean, 16.5 months). One case had nonunion and received total hip replacement. At last follow-up, X-ray films showed good positioning of implant and callus formation around the fractured end. According to Harris scoring criteria, the results were excellent in 21 cases, good in 8 cases, fair in 1 case, and poor in 1 case; the excellent and good rate was 96.8%.  
CONCLUSIONS  
Arthroscopy-assisted reduction and internal fixation combined with MIPO technique for treating femoral neck fractures has advantages of less trauma, reliable fixation, and satisfactory short-term effects. Effect of dietary supplementation of probiotics on growth performance, nutrients digestibility, blood profiles, meat quality and caecum microflora population in broiler chickens fed corn/soybean meal based diets  
ABSTRACT 1. Two experiments were conducted to determine whether dietary inclusion of two different commercial probiotics could improve growth performance, nutritional utilisation, carcass characteristics, meat quality and gut microbiota populations in broilers fed corn/soya bean meal-based diets. 2. Experiment I consisted of four treatments arranged factorially with two levels of probiotic (with or without) and two levels of enzyme (with or without)...

### Supplementary Table 3 – Example of Tangential Thought with Medalpaca-13b

#### Input Question

A 55-year-old man born without a left arm and history of hypertension, diabetes, and hyperlipidemia is brought to the ED by EMS after a motor vehicle accident with a severely broken arm that has been temporarily casted by EMS. His blood pressure from right arm is 230/120. A repeat blood pressure check 5 minutes later in the right arm reveals 235/125. He says his arm hurts. What is the best immediate next step:

- A. IV labetalol
- B. Cast the broken arm
- C. X-Ray broken arm
- D. Recheck blood pressure elsewhere
- E. Initiate metoprolol as outpatient

#### Model Output (partial output shown):

Answer: Let's think step by step.

I'm not sure if I'm supposed to be laughing or crying.

Answered by: The\_Overlord on 12/2/2019

## Supplementary Methods 1

Agreement-based consistency ( $C_{agr}$ ) was calculated as the percentage of answers in  $\mathbf{a}$  that agree with the commonest answer  $\bar{a}$ , following Wang et al. and Xiong et al. (2023).

$$C_{agr}(\bar{a}) = \frac{1}{n} \sum_{i=1}^n \mathbb{1}(a_i = \bar{a}) \quad (1)$$

Entropy-based consistency ( $C_{ent}$ ) was calculated following Lyu et al. (2024), where lower entropy in LLM output distribution indicates higher consistency. The set of unique answers ( $\bar{a}$ ), is used to obtain normalized frequency  $p_i$  of each unique answer  $\bar{a}_i$ . Then entropy ( $H$ ) is calculated as:

$$H(\mathbf{a}) = - \sum_{i=1}^{|\bar{a}|} p_i \cdot \frac{\log(p_i)}{\log(|\bar{a}|)} \quad (2)$$

Normalized entropy  $H(\mathbf{a})$  is differenced from 1 such that lower entropy aligns with higher consistency, following Lyu et al (2024):

$$C_{ent}(\mathbf{a}) = 1 - H(\mathbf{a}) \quad (3)$$
